# Supplementary material for: From superdeformation to extreme deformation and clusterization in the N~Z nuclei of the A~40 mass region
Source: arXiv:1606.04019 source file (2016-06-13)
Supplement: Supplementary file 1 [file supplement.pdf]

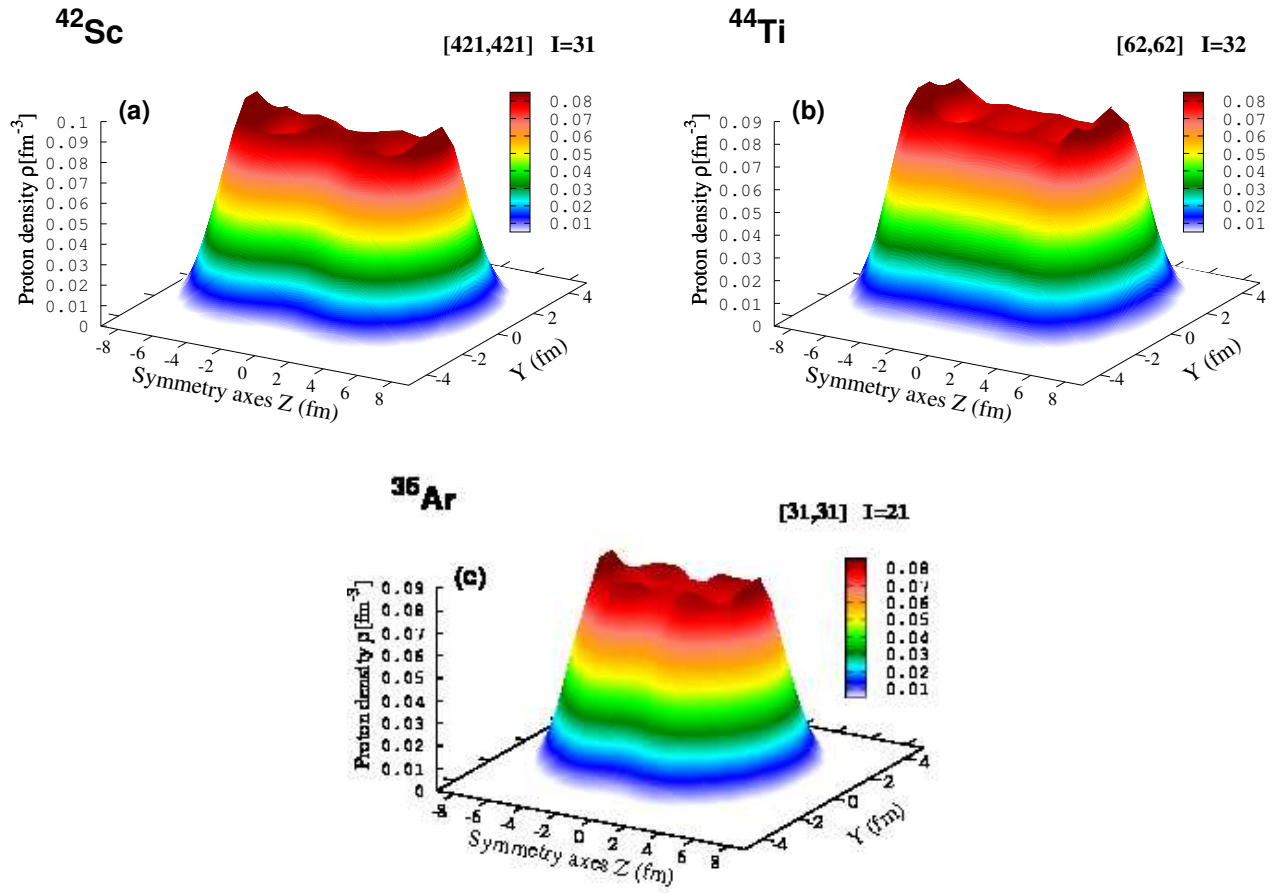

FIG. 1. (Color online) Three-dimensional representation of proton densities in the indicated configurations of  $^{42}\text{Sc}$ ,  $^{44}\text{Ti}$  and  $^{36}\text{Ar}$ .

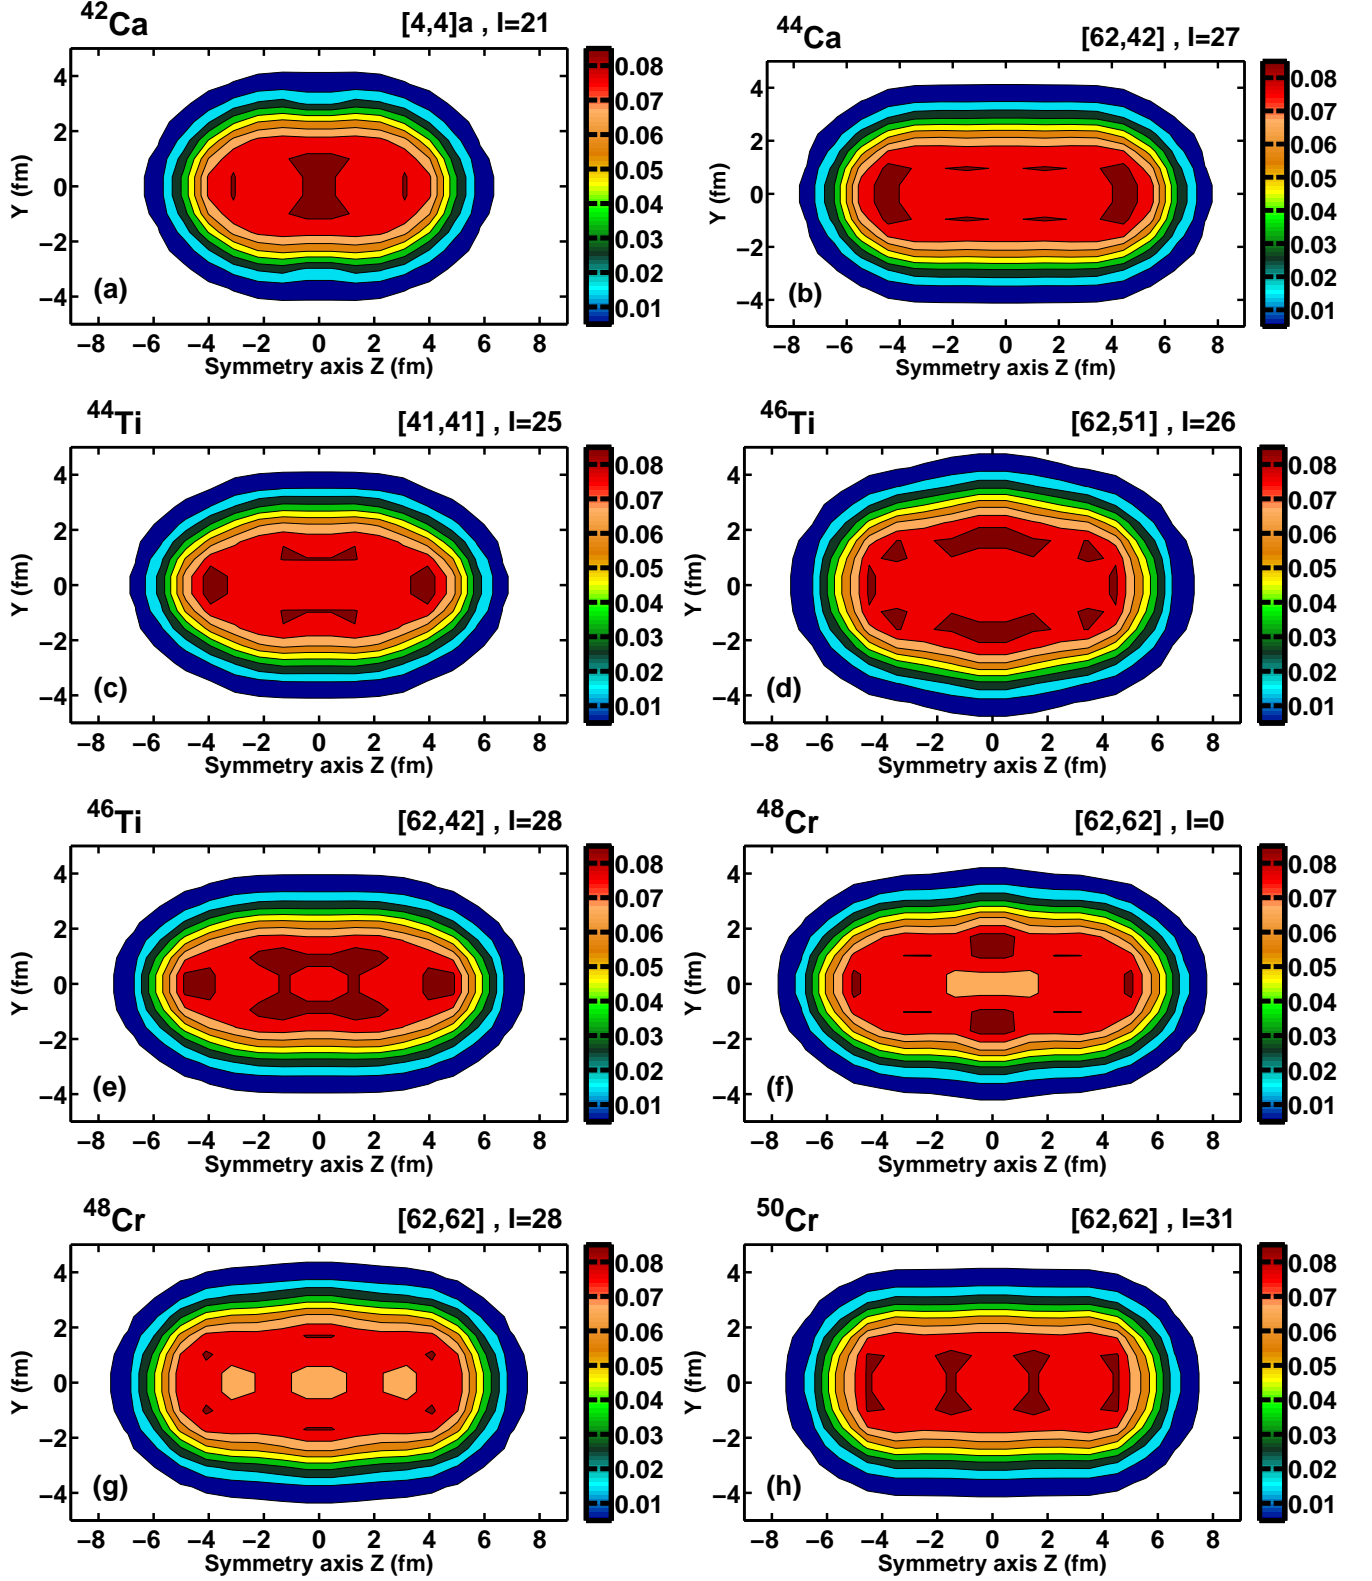

FIG. 2. (Color online) The self-consistent proton density  $\rho_p(y, z)$  as a function of  $y$  and  $z$  coordinates for the indicated configurations of selected nuclei at specified spin values. The equidensity lines are shown in steps of  $0.01 \text{ fm}^{-3}$  starting from  $\rho_p(y, z) = 0.01 \text{ fm}^{-3}$ .

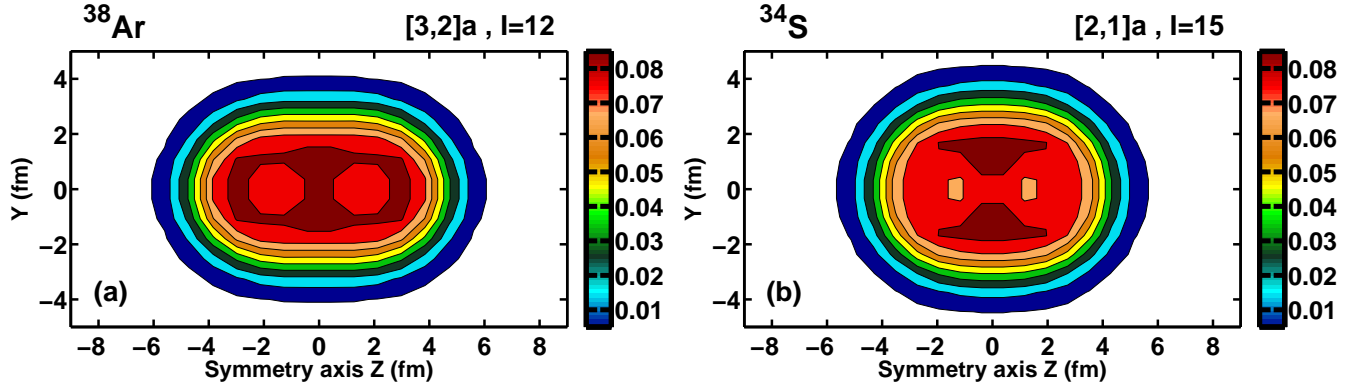

FIG. 3. (Color online) The same as Fig. 2 but for  $^{38}\text{Ar}$  and  $^{34}\text{S}$ .

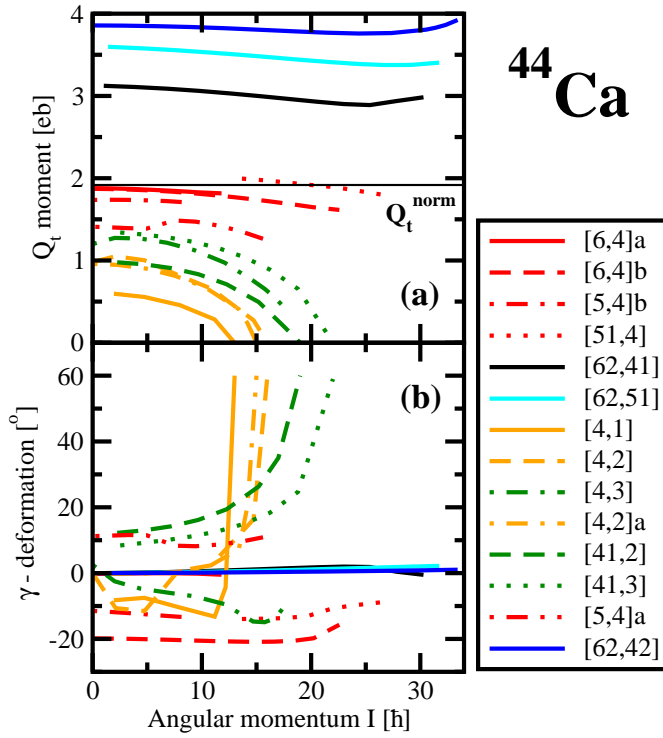

FIG. 4. (Color online) Calculated transition quadrupole moments  $Q_t$  and  $\gamma$ -deformations of the yrast and excited SD and HD configurations in  $^{44}\text{Ca}$ . The colors of the lines for different types of configurations roughly correspond to those used in  $E - E_{RLD}$  plots of the main body of the manuscript.

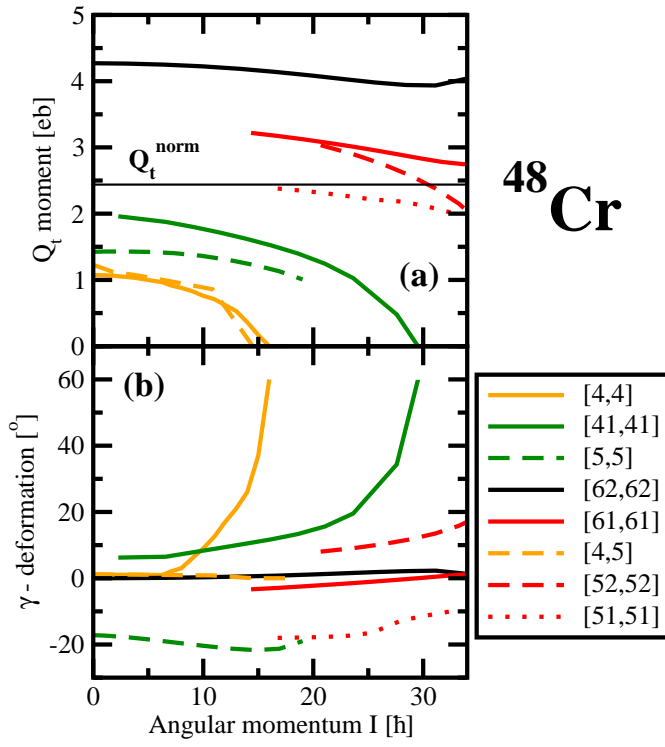

FIG. 5. (Color online) The same as Fig. 4 but for  $^{48}\text{Cr}$ .

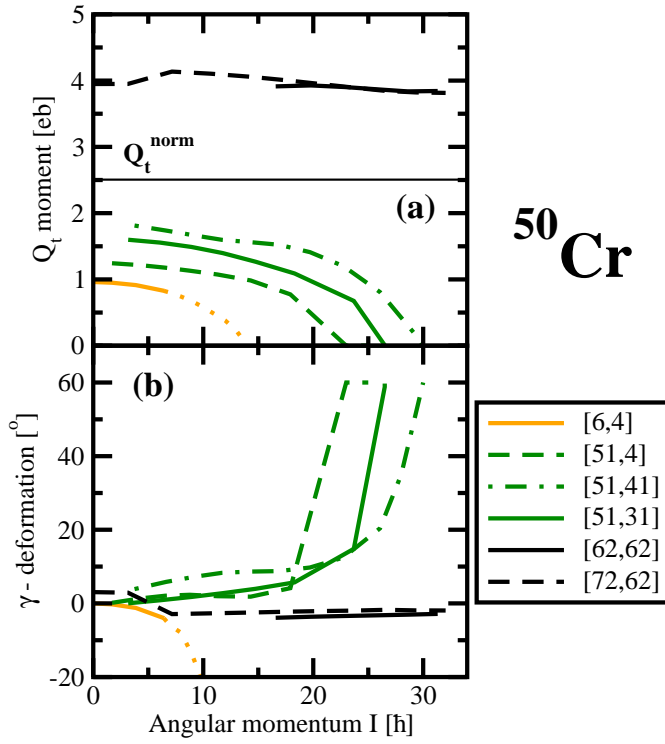

FIG. 6. (Color online) The same as Fig. 4 but for  $^{50}\text{Cr}$ .

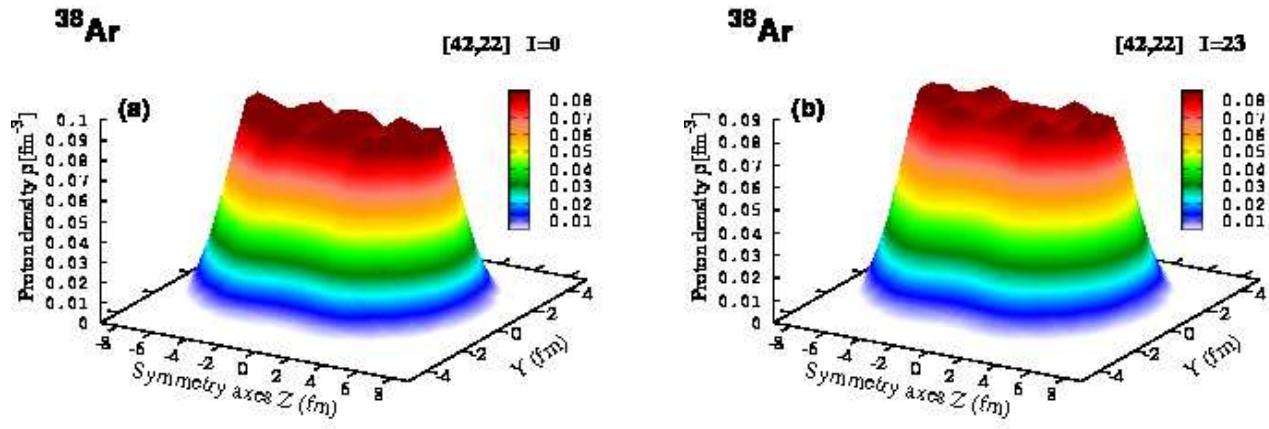

FIG. 7. (Color online) Three-dimensional representation of the evolution of proton density distribution with spin in the the  $[42,22]$  configuration in  $^{38}\text{Ar}$ .
